# Supplementary material for: Elastic weight consolidation for better bias inoculation
Source: arXiv:2004.14366 source file (2021-02-04)
Supplement: Supplementary file 1 [file supplementary.tex]

\documentclass[11pt,a4paper]{article}
\usepackage[hyperref]{eacl2021}
\usepackage{times}
\usepackage{amsmath}
\usepackage{amsfonts}
\usepackage{latexsym}
\usepackage{booktabs}
\usepackage{url}
\usepackage{tikz}
\usepackage{multirow}
\usepackage{qtree}
\usepackage{float}
\usepackage{tikz-cd}
\usepackage{pgfplots}
\usepackage[]{todonotes}
\usepackage[caption=false]{subfig}

%\aclfinalcopy

\pgfplotsset{every axis/.append style={
                    label style={font=\footnotesize},
                    tick label style={font=\footnotesize} 
                    }}

%\title{Avoiding catastrophic forgetting when mitigating NLI model biases}
\title{Supplementary Materials}
%AV: I don't like it much, but feels better than not narrowing the scope of the title given what follows.
\author{James Thorne \\
  Department of Computer Science \\
  University of Cambridge \\
  {\tt jt719@cam.ac.uk} \\\And
  Andreas Vlachos \\
  Department of Computer Science \\
  University of Cambridge \\
  {\tt av308@cam.ac.uk} \\}

\date{}

\begin{document}
\maketitle

\input{appendix}

\bibliography{refs2}
\bibliographystyle{acl_natbib}

\end{document}
